# Supplementary material for: Calibration of Large Language Models on Code Summarization
Source: arXiv:2404.19318 source file (2025-05-30)
Supplement: Supplementary file 1 [file supplementary.tex]

%\begin{table*}[t]
\begin{table*}[t!]
\centering
\resizebox{.98\textwidth}{!}{%
\begin{tabular}{lllrrrrrrrrr}
\toprule
 &  &  & BERT Score & BLEU-1 & Infersent-CS & ROUGE-1-P & ROUGE-4-R & ROUGE-W-R & SIDE & Sentence BERT \\
Language & Model & Prompt &  &  &  &  &  &  &  &  &  \\
\midrule
\multirow[t]{6}{*}{Java} & \multirow[t]{2}{*}{CodeLlama-70b-hf} & ASAP & 0.34 & 0.52 & 0.72 & 0.47 & 0.16 & 0.34 & 0.76 & 0.64 \\
 &  & BM25 & 0.33 & 0.52 & 0.71 & 0.47 & 0.13 & 0.31 & 0.78 & 0.63 \\
\cline{2-12}
 & \multirow[t]{2}{*}{deepseek-coder-33b-instruct} & ASAP & 0.32 & 0.51 & 0.72 & 0.46 & 0.11 & 0.32 & 0.83 & 0.63 \\
 &  & BM25 & 0.32 & 0.49 & 0.70 & 0.45 & 0.10 & 0.30 & 0.83 & 0.62 \\
\cline{2-12}
 & \multirow[t]{2}{*}{gpt-3.5-turbo} & ASAP & 0.33 & 0.53 & 0.73 & 0.51 & 0.10 & 0.24 & 0.68 & 0.63 \\
 &  & BM25 & 0.31 & 0.49 & 0.72 & 0.53 & 0.06 & 0.17 & 0.55 & 0.60 \\
\cline{1-12} \cline{2-12}
\multirow[t]{6}{*}{Python} & \multirow[t]{2}{*}{CodeLlama-70b-hf} & ASAP & 0.31 & 0.51 & 0.69 & 0.45 & 0.14 & 0.34 & 0.36 & 0.61 \\
 &  & BM25 & 0.31 & 0.51 & 0.71 & 0.44 & 0.10 & 0.32 & 0.31 & 0.61 \\
\cline{2-12}
 & \multirow[t]{2}{*}{deepseek-coder-33b-instruct} & ASAP & 0.31 & 0.52 & 0.71 & 0.45 & 0.09 & 0.31 & 0.28 & 0.62 \\
 &  & BM25 & 0.30 & 0.49 & 0.70 & 0.43 & 0.07 & 0.30 & 0.29 & 0.60 \\
\cline{2-12}
 & \multirow[t]{2}{*}{gpt-3.5-turbo} & ASAP & 0.26 & 0.51 & 0.70 & 0.46 & 0.04 & 0.18 & 0.32 & 0.57 \\
 &  & BM25 & 0.26 & 0.51 & 0.71 & 0.46 & 0.04 & 0.18 & 0.33 & 0.58 \\
\cline{1-12} \cline{2-12}
\bottomrule
\end{tabular}
}
\caption{Model Benchmarks}
\end{table*}

\begin{figure*}
  \centering
  \captionsetup{font=small} 

  \begin{subfigure}[t]{0.3\linewidth}
    \includegraphics[width=\linewidth]{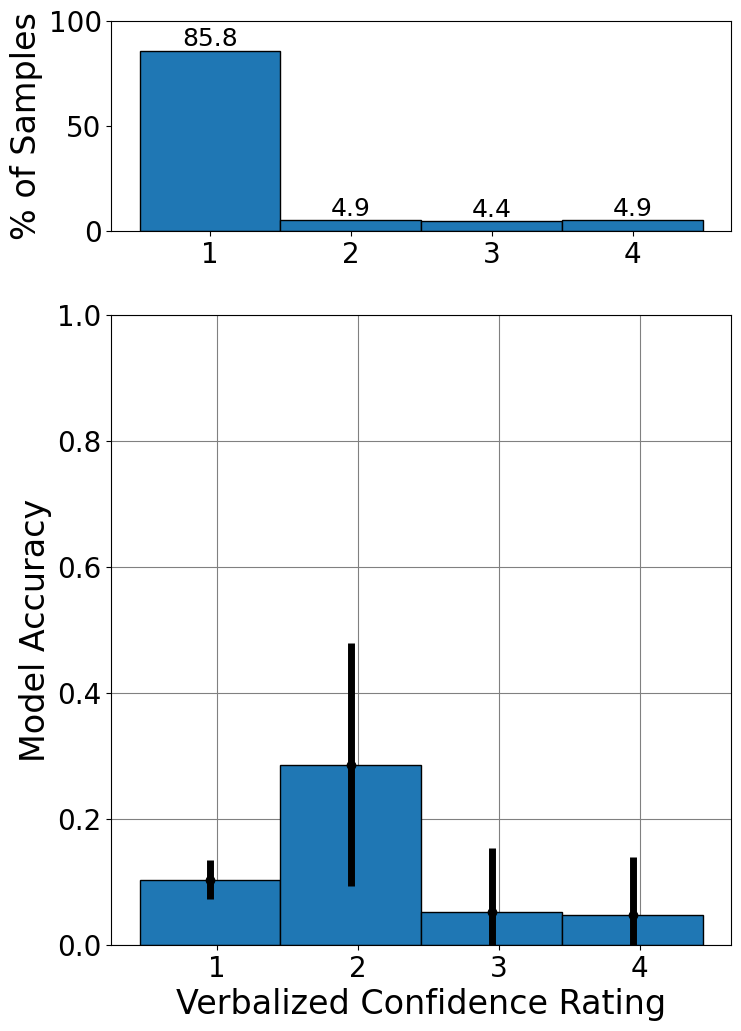}
    \caption{deepseek-coder-33b-instruct Java}
    \label{fig:figure9a}
  \end{subfigure}
  \hspace{5pt}
  \begin{subfigure}[t]{0.3\linewidth}
    \includegraphics[width=\linewidth]{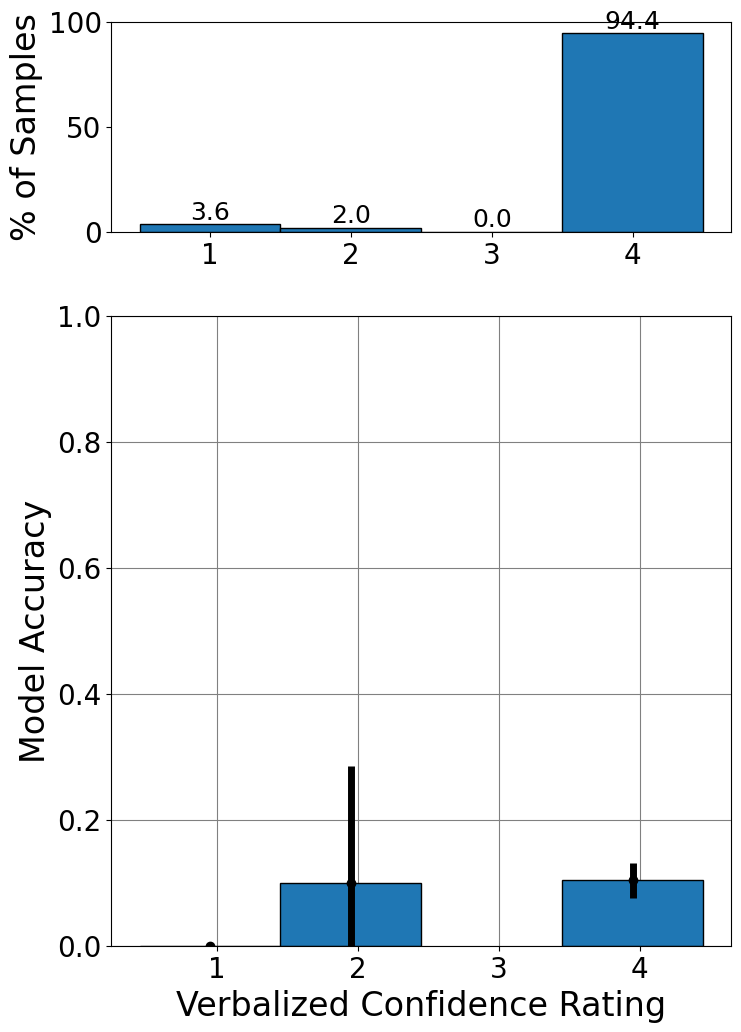}
    \caption{GPT-3.5 Turbo on Java}
    \label{fig:figure9b}
  \end{subfigure}
  \hspace{5pt}
  \begin{subfigure}[t]{0.3\linewidth}
    \includegraphics[width=\linewidth]{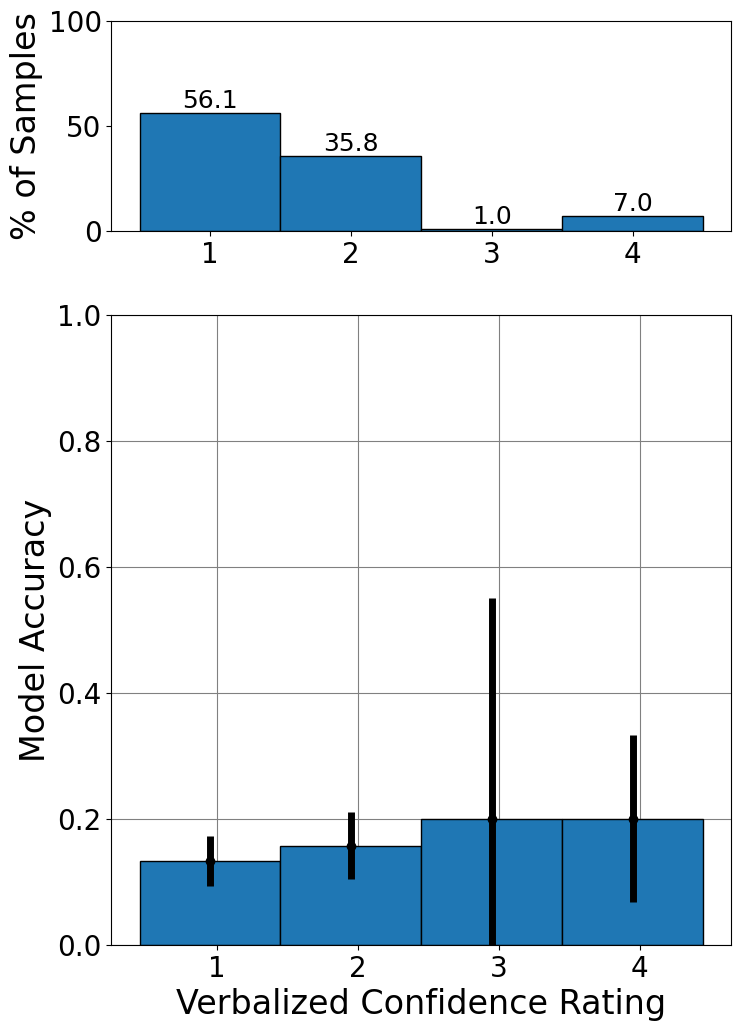}
    \caption{GPT-3.5 Turbo on Java}
    \label{fig:figure9b}
  \end{subfigure}
  \hspace{5pt}
  \caption{4-shot Verbalized Confidence}
  \label{fig:grid-comparison}
\end{figure*}
